# Supplementary material for: Switching Nonparametric Regression Models and the Motorcycle Data revisited
Source: arXiv:1305.2227 ancillary file (2013-05-22)
Supplement: Supplementary file 1 [file DeSouzaHeckman-supplementA.pdf]

# Switching Nonparametric Regression Models and the Motorcycle Data revisited

# Supplementary Material

Camila P. E. de Souza and Nancy E. Heckman

## 1 The proposed EM algorithm

We will use an EM algorithm to find $\hat{\theta}$ that maximizes

$$l(\theta) \quad = \quad \log p(\mathbf{y}|\theta) + P(f_1, \ldots, f_J, \lambda_1, \ldots, \lambda_J), \tag{1}$$

where $\log p(\mathbf{y}|\theta)$ and $P(f_1, \ldots, f_J, \lambda_1, \ldots, \lambda_J)$ are as in Section 4 of the paper.

The derivation of the EM algorithm can be summarized in two steps:

1. $l(\theta)$ is expressed in terms of the latent data;

2. We use this expression to come up with a sequence of $\theta^{(c)}$'s which will not decrease $l(\theta)$, that is, with $l(\theta^{(c+1)}) - l(\theta^{(c)}) \geq 0$.

The joint distribution of $\mathbf{y}$ and $\mathbf{z}$ (also called the complete data distribution) can be written as $p(\mathbf{y}, \mathbf{z}|\theta) = p(\mathbf{z}|\mathbf{y}, \theta)p(\mathbf{y}|\theta)$. Rearranging this we get that, for any $\mathbf{z}$ with $p(\mathbf{z}|\mathbf{y}, \theta) > 0$,

$$p(\mathbf{y}|\theta) = \frac{p(\mathbf{y}, \mathbf{z}|\theta)}{p(\mathbf{z}|\mathbf{y}, \theta)}.$$

Taking the logarithm we have $\log p(\mathbf{y}|\theta) = \log p(\mathbf{y}, \mathbf{z}|\theta) - \log p(\mathbf{z}|\mathbf{y}, \theta)$ and, substituting this in (1), we get

$$l(\theta) = \log p(\mathbf{y}, \mathbf{z}|\theta) - \log p(\mathbf{z}|\mathbf{y}, \theta) + P(f_1, \ldots, f_J, \lambda_1, \ldots, \lambda_J). \tag{2}$$

Multiplying both sides of (2) by $p(\mathbf{z}|\mathbf{y}, \theta^{(c)})$ and summing over all possible values of $\mathbf{z}$ preserves the equality. The left side is unchanged, since $l(\theta)$ does not depend on $\mathbf{z}$. Since the

penalty term $P(f_1, \ldots, f_J, \lambda_1, \ldots, \lambda_J)$ does not depend on $\mathbf{z}$ the right hand side of (2) becomes

$$\sum_{\mathbf{z}} \log p(\mathbf{y}, \mathbf{z}|\theta) p(\mathbf{z}|\mathbf{y}; \theta^{(c)}) - \sum_{\mathbf{z}} \log p(\mathbf{z}|\mathbf{y}, \theta) p(\mathbf{z}|\mathbf{y}; \theta^{(c)}) + P(f_1, \ldots, f_J, \lambda_1, \ldots, \lambda_J),$$

Therefore, we can write

$$l(\theta) = Q(\theta, \theta^{(c)}) - H(\theta, \theta^{(c)}) + P(f_1, \ldots, f_J, \lambda_1, \ldots, \lambda_J), \tag{3}$$

where

$$Q(\theta, \theta^{(c)}) = \sum_{\mathbf{z}} \log p(\mathbf{y}, \mathbf{z}|\theta) p(\mathbf{z}|\mathbf{y}; \theta^{(c)})$$

and

$$H(\theta, \theta^{(c)}) = \sum_{\mathbf{z}} \log p(\mathbf{z}|\mathbf{y}, \theta) p(\mathbf{z}|\mathbf{y}; \theta^{(c)}).$$

Consider equation (3) and let $S(\theta, \theta^{(c)}) = Q(\theta, \theta^{(c)}) + P(f_1, \ldots, f_J, \lambda_1, \ldots, \lambda_J)$. Finding a value $\theta^{(c+1)}$ so that $l(\theta^{(c+1)}) \geq l(\theta^{(c)})$ is the same as finding $\theta^{(c+1)}$ so that

$$S(\theta^{(c+1)}, \theta^{(c)}) - S(\theta^{(c)}, \theta^{(c)}) - H(\theta^{(c+1)}, \theta^{(c)}) + H(\theta^{(c)}, \theta^{(c)}) \geq 0. \tag{4}$$

Note that for any $\theta$

$$\begin{aligned} H(\theta, \theta^{(c)}) - H(\theta^{(c)}, \theta^{(c)}) &= \mathrm{E}_{\theta^{(c)}}(\log\{p(\mathbf{z}|\mathbf{y}, \theta)/p(\mathbf{z}|\mathbf{y}, \theta^{(c)})\}|\mathbf{y}) \\ &\leq \log\left[\mathrm{E}_{\theta^{(c)}}\{p(\mathbf{z}|\mathbf{y}, \theta)/p(\mathbf{z}|\mathbf{y}, \theta^{(c)})\}|\mathbf{y}\right] \qquad (5) \\ &= \log \sum_{\mathbf{z}} \frac{p(\mathbf{z}|\mathbf{y}, \theta)}{p(\mathbf{z}|\mathbf{y}, \theta^{(c)})} p(\mathbf{z}|\mathbf{y}, \theta^{(c)}) \\ &= \log \sum_{\mathbf{z}} p(\mathbf{z}|\mathbf{y}, \theta) = \log 1 \\ &= 0, \end{aligned}$$

where the inequality in (5) is a consequence of Jensen's inequality and the concavity of the logarithmic function.

Therefore, we can guarantee that (4) holds if we guarantee that $S(\theta^{(c+1)}, \theta^{(c)}) - S(\theta^{(c)}, \theta^{(c)}) \geq 0$. To do that choose $\theta^{(c+1)}$ as any value of $\theta$ which does not decrease $S(\theta, \theta^{(c)})$ for the current value at $\theta^{(c)}$. If $\theta^{(c+1)}$ is the maximizing value, then $S(\theta^{(c+1)}, \theta^{(c)}) \geq S(\theta^{(c)}, \theta^{(c)})$.

To increase the rate of convergence of the algorithm we recommend taking

$$\theta^{(c+1)} = \arg\max_{\theta} S(\theta, \theta^{(c)}) \text{ if possible.}$$

More details on the EM algorithm can be found in McLachlan and Krishnan (2008).

# 2 The ECM algorithm

Sometimes the M-step of the EM algorithm is complicated and, therefore, this algorithm becomes less atractive. In many cases, however, the M-step becomes relatively simple if the maximization is undertaken conditional on some of the parameters (or some functions of the parameters). Meng and Rubin (1993) use this idea in an extension to the EM algorithm, which they call the ECM algorithm for expectation-conditional maximization algorithm. The ECM algorithm replaces a complicated M-step of the EM algorithm with several computationally simpler conditional maximization steps (CM-steps). In our case, each CM-step maximizes $S(\theta, \theta^{(c)}) = Q(\theta, \theta^{(c)}) + P(f_1, \ldots, f_J, \lambda_1, \ldots, \lambda_J)$ subject to constraints on the set of parameters $\theta$, where the collection of all constraints is such that the maximization is over the full parameter space of $\theta$.

## 2.1 Formal definition

Instead of updating $\theta^{(c)}$ to $\theta^{(c+1)}$ directly via one M-step, we replace the M-step by $R > 1$ CM-steps. Let $\theta^{(c+r/R)}$ denote the value of $\theta$ on the $r$th CM-step of the update, where $\theta^{(c+r/R)}$ is the value that maximizes $S(\theta, \theta^{(c)})$ subject to the constraint

$$\mathbf{g}_r(\theta) = \mathbf{g}_r(\theta^{(c+(r-1)/R)}).$$

Here, $\{\mathbf{g}_r(\theta), r = 1, \ldots, R\}$ is a set of preselected vector-valued functions. Thus, $\theta^{(c+r/R)}$ satisfies

$$S(\theta^{(c+r/R)}, \theta^{(c)}) \geq S(\theta, \theta^{(c)}) \text{ for all } \theta \text{ such that } \mathbf{g}_r(\theta) = \mathbf{g}_r(\theta^{(c+(r-1)/R)}). \tag{6}$$

In particular $S(\theta^{(c+r/R)}, \theta^{(c)}) \geq S(\theta^{(c+(r-1)/R)}, \theta^{(c)})$.

The value of $\theta$ on the final CM-step, $\theta^{(c+R/R)} = \theta^{(c+1)}$, is taken to be the input for the next iteration. From (6) we have

$$S(\theta^{(c+1)}, \theta^{(c)}) \geq S(\theta^{(c+(R-1)/R)}, \theta^{(c)}) \geq S(\theta^{(c+(R-2)/R)}, \theta^{(c)}) \geq \cdots \geq S(\theta^{(c)}, \theta^{(c)}).$$

As noted before in Section 1 of this supplement, this inequality is a sufficient condition for $l(\theta^{(c+1)}) \geq l(\theta^{(c)})$ to hold. This shows that the ECM algorithm has the same desirable convergence properties as the EM algorithm.

## 2.2 Example

Consider the M-step presented in Section 4.2 of the paper for *iid* $z_i$'s. We want to increase the value of $S(\theta, \theta^{(c)})$ with respect to $\theta = \{p_j, \sigma_j^2, f_j(\mathbf{x})\}$ from the value at $\theta = \theta^{(c)}$. In this case we have a total of $R = 3$ CM-steps described as follows.

$r = 1$:

Let $\mathbf{g}_1(p_j, \sigma_j^2, f_j(\mathbf{x}))$ be a partition of $\theta$, that is, $\mathbf{g}_1(p_j, \sigma_j^2, f_j(\mathbf{x})) = \{p_j, \sigma_j^2\}$. Thus, we want to maximize $S(\theta, \theta^{(c)})$ over $\theta$ subject to

$$\mathbf{g}_1(p_j, \sigma_j^2, f_j(\mathbf{x})) = \mathbf{g}_1(p_j^{(c)}, \sigma_j^{2\,(c)}, f_j(\mathbf{x})^{(c)}),$$

i.e., maximize $S(\theta, \theta^{(c)})$ over $f_j(\mathbf{x})$ holding $p_j = p_j^{(c)}$ and $\sigma_j^2 = \sigma_j^{2\,(c)}$. As a result we obtain

$$\theta^{(c+1/R)} = \{p_j^{(c+1/3)}, \sigma_j^{2\,(c+1/3)}, f_j(\mathbf{x})^{(c+1/3)}\} = \{p_j^{(c)}, \sigma_j^{2(c)}, \hat{f}_j(\mathbf{x})\}, \tag{7}$$

where $\hat{f}_j(\mathbf{x}) = \mathbf{H}_j\mathbf{y}$. The form of the hat matrix $\mathbf{H}_j$ depends on the approach considered (Bayesian or penalized log-likelihood).

$r = 2$:

Let $\mathbf{g}_2(p_j, \sigma_j^2, f_j) = \{p_j, f_j(\mathbf{x})\}$. We want to maximize $S(\theta, \theta^{(c)})$ over $\theta$ subject to

$$\mathbf{g}_2(p_j, \sigma_j^2, f_j) = \mathbf{g}_2(p_j^{(c+1/3)}, \sigma_j^{2\,(c+1/3)}, f_j^{(c+1/3)}),$$

i.e., maximize $S(\theta, \theta^{(c)})$ over $\sigma_j^2$ holding $p_j = p_j^{(c+1/3)} = p_j^{(c)}$ and $f_j(\mathbf{x}) = f_j(\mathbf{x})^{(c+1/3)} = \hat{f}_j(\mathbf{x})$. As a result we obtain

$$\theta^{(c+2/3)} = \{p_j^{(c+2/3)}, \sigma_j^{2\,(c+2/3)}, f_j(\mathbf{x})^{(c+2/3)}\} = \{p_j^{(c)}, \hat{\sigma}_j^2, \hat{f}_j(\mathbf{x})\}, \tag{8}$$

where $\hat{\sigma}_j^2 = \sum_{i=1}^n \left[(y_i - \hat{f}_j(x_i))^2 \times p_{ij}^{(c)}\right] / \left[\sum_{i=1}^n p_{ij}^{(c)} - \mathrm{trace}(\mathbf{H}_j)\right]$.

$r = 3$:

Let $\mathbf{g}_3(p_j, \sigma_j^2, f_j) = \{\sigma_j^2, f_j(\mathbf{x})\}$. We want to maximize $S(\theta, \theta^{(c)})$ over $\theta$ subject to

$$\mathbf{g}_3(p_j, \sigma_j^2, f_j) = \mathbf{g}_3(p_j^{(c+2/3)}, \sigma_j^{2\,(c+2/3)}, f_j^{(c+2/3)}),$$

i.e., maximize $S(\theta, \theta^{(c)})$ over $p_j$ holding $\sigma_j^2 = \sigma_j^{2\,(c+2/3)} = \hat{\sigma}_j^2$ and $f_j(\mathbf{x}) = f_j(\mathbf{x})^{(c+2/3)} = \hat{f}_j(\mathbf{x})$. As a result we obtain

$$\theta^{(c+3/3)} = \theta^{(c+1)} = \{\hat{p}_j^{(c+1)}, \sigma_j^{2\,(c+1)}, f_j(\mathbf{x})^{(c+1)}\} = \{\hat{p}_j, \hat{\sigma}_j^2, \hat{f}_j(\mathbf{x})\}, \tag{9}$$

where $\hat{p}_j = \sum_{i=1}^n p_{ij}^{(c)}/n$.

More examples and details about the ECM algorithm can be found in McLachlan and Krishnan (2008).

# References

McLachlan, G. and Krishnan, T. (2008), *The EM Algorithm and Extensions*, 2nd Ed., Wiley New York.

Meng, X. and Rubin, D. (1993), "Maximum likelihood estimation via the ECM algorithm: a general framework," *Biometrika*, 80, 267–278.
